# Supplementary material for: EIC Physics from An All-Silicon Tracking Detector
Source: arXiv:2102.08337 source file (2021-02-16)

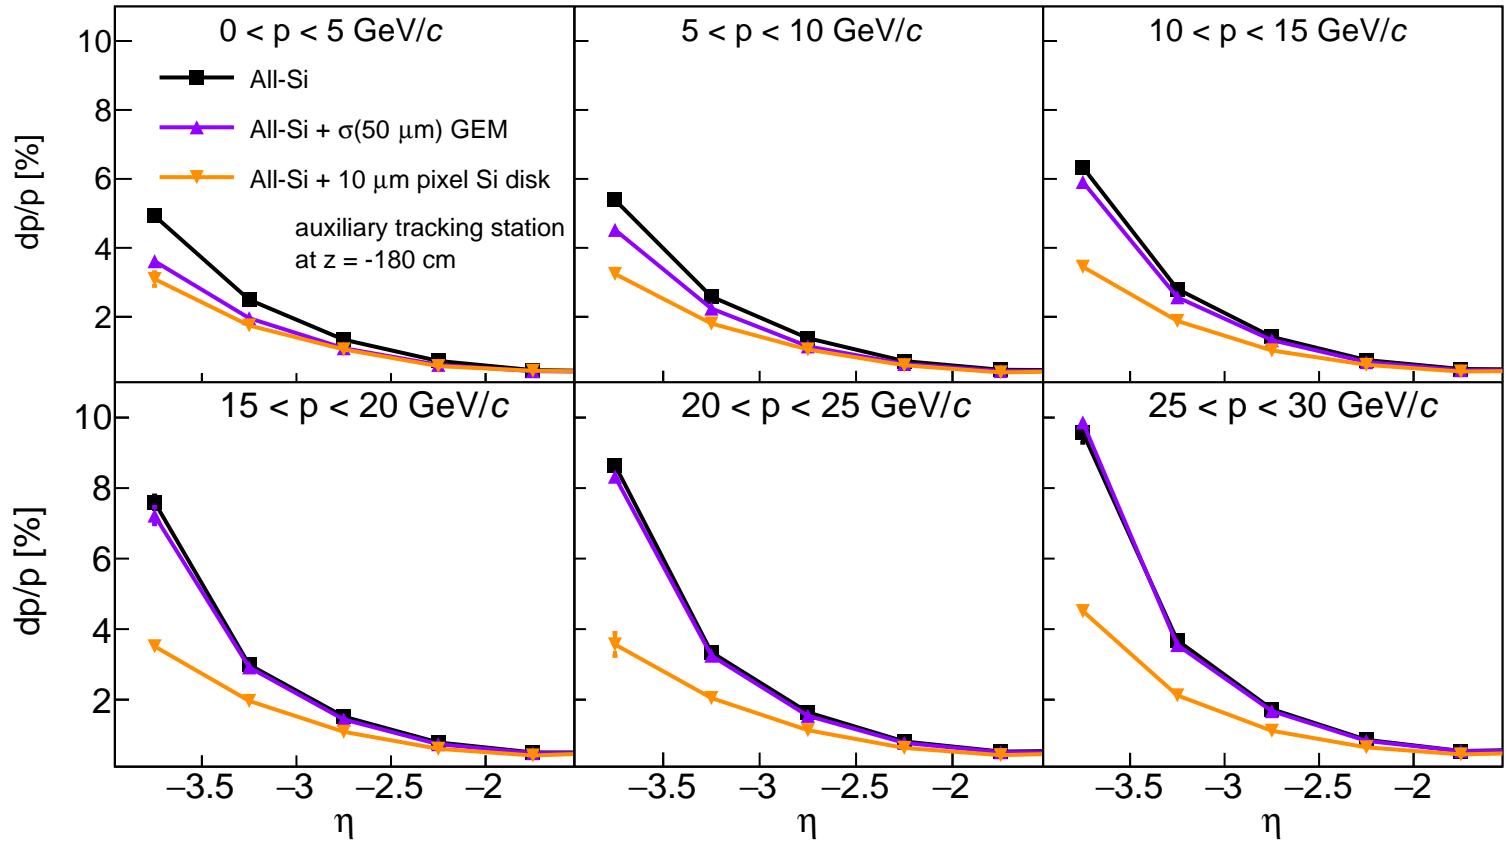

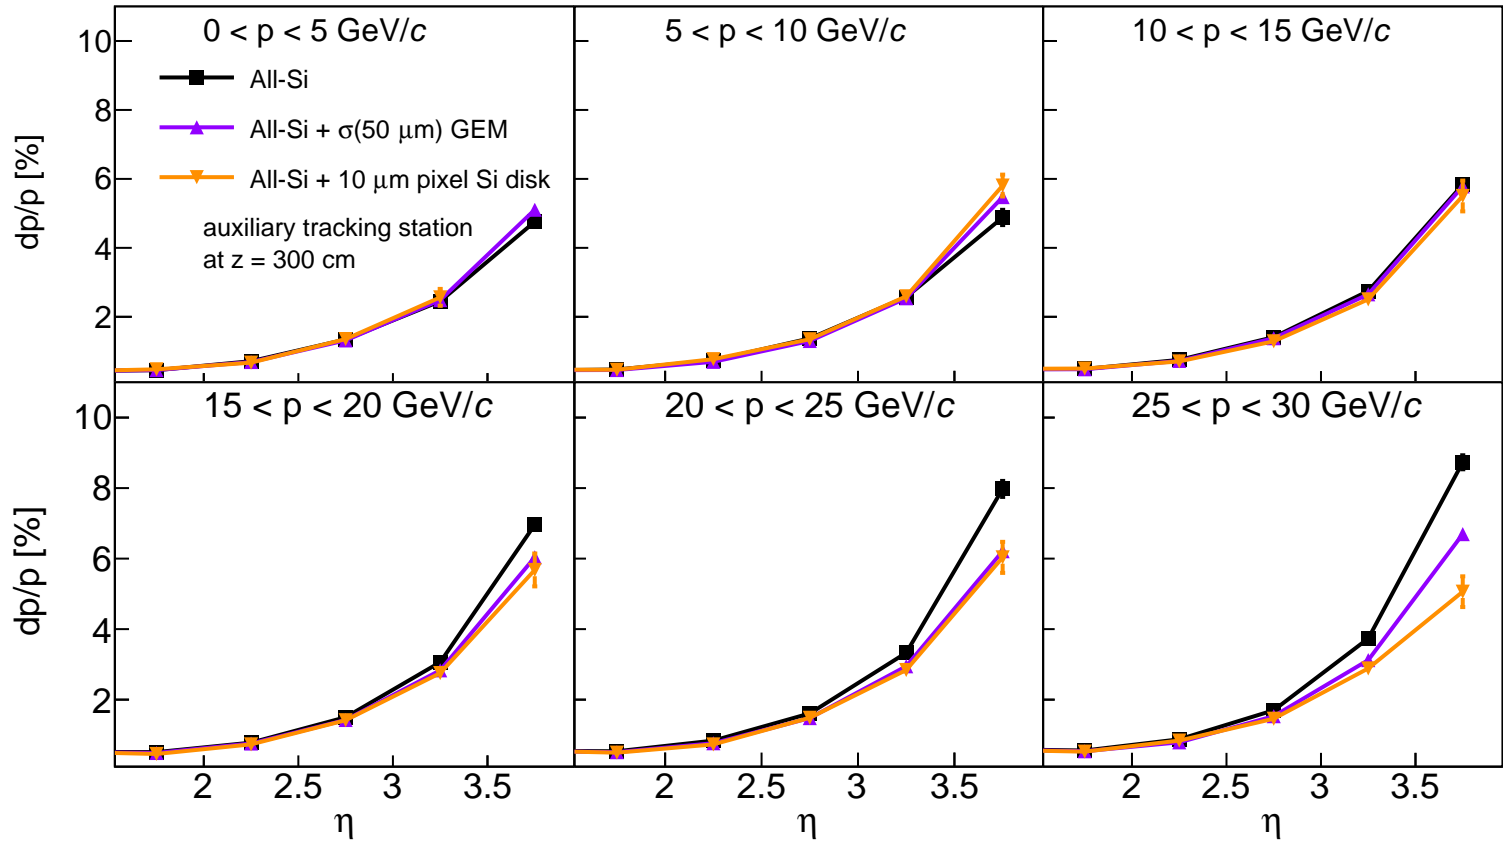

Supplement: Supplementary file 1 [file all_si_GEM_si_disk.pdf]
